# Supplementary material for: Deterministic hBN bubbles as a versatile platform for studies on single-photon emitters
Source: arXiv:2510.11610 source file (2025-10-13)
Supplement: Supplementary file 1 [file SI.pdf]

# Supporting Information for Deterministic hBN bubbles as a versatile platform for studies on single-photon emitters

Piotr Tatarczak,* Tomasz Fąs, Jan Pawłowski, Aleksandra Krystyna Dąbrowska, Jan Suffczyński, Piotr Wróbel, Andrzej Wysmołek,* and Johannes Binder

*Faculty of Physics, University of Warsaw, ul. Pasteura 5, 02-093 Warsaw*

E-mail: Piotr.Tatarczak@fuw.edu.pl; Andrzej.Wysmolek@fuw.edu.pl

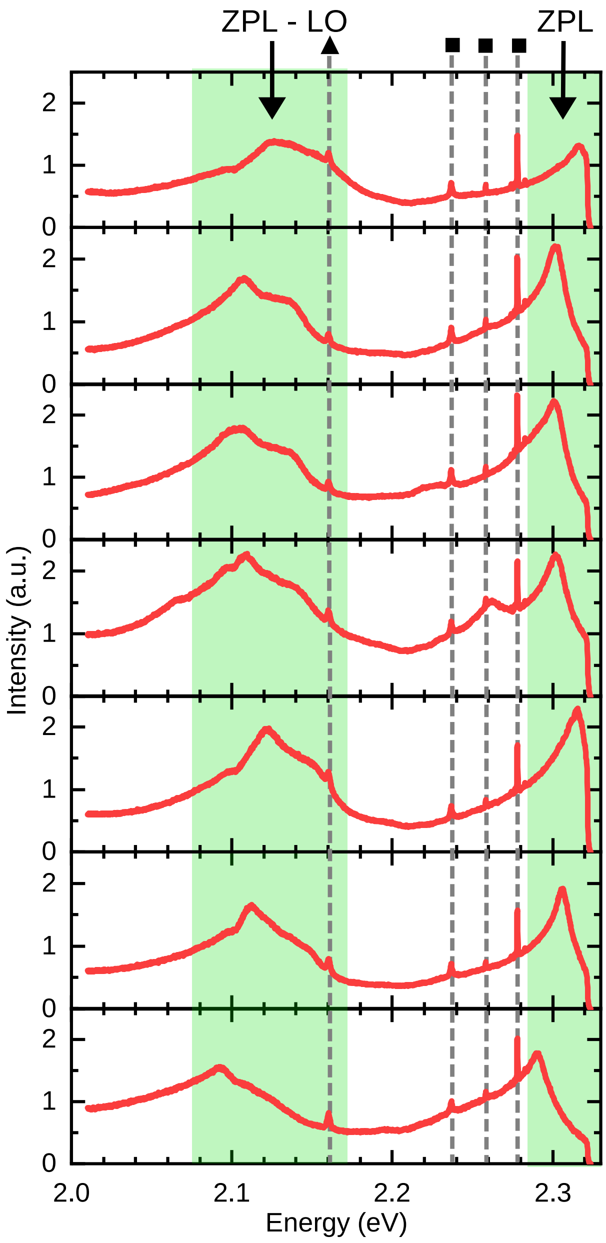


Figure S1: Typical spectra exhibiting defect-related emission across the flat non-bubbled hBN. ZPLs and their phonon replica are marked by green color and arrows. Vibrational modes of sapphire (hBN) are indicated by gray dashed lines and black squares (triangle).

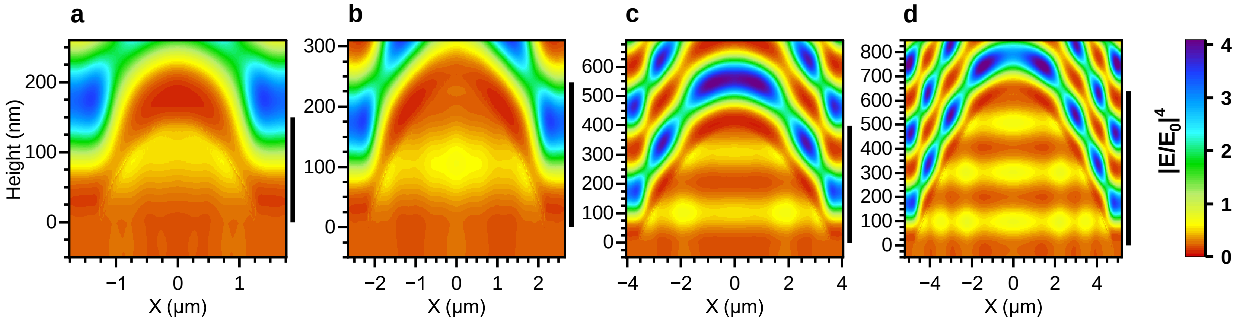


Figure S2: Simulations of $|E/E_0|^4$ distribution near bubbles B1-B4. The top surface of the sapphire substrate is placed at 0 nm in the height scale. Black lines on the right sides of panels indicate bubble heights.

Figure S1 presents typical spectra acquired in flat hBN that was not irradiated by electrons. Characteristic ZPLs at ∼2.3 eV and phonon replicas (ZPL-LO) at ∼2.1 eV are observed. In all cases, the maximum intensity is around 2-4 times smaller than the intensity of SPEs found on bubbles.

Figure S2 presents detailed simulations of the distribution of $|E/E_0|^4$ ($E$ - local electric field, $E_0$ - electric field of the incident light) in bubble surroundings. In contrast to the values in the Figure. 6e-h, here $|E/E_0|^4$ is not normalized, but real values are shown. In all cases, interference-like maxima are formed due to bubble geometries, leading to enhanced intensity of Raman and defect-related emission.

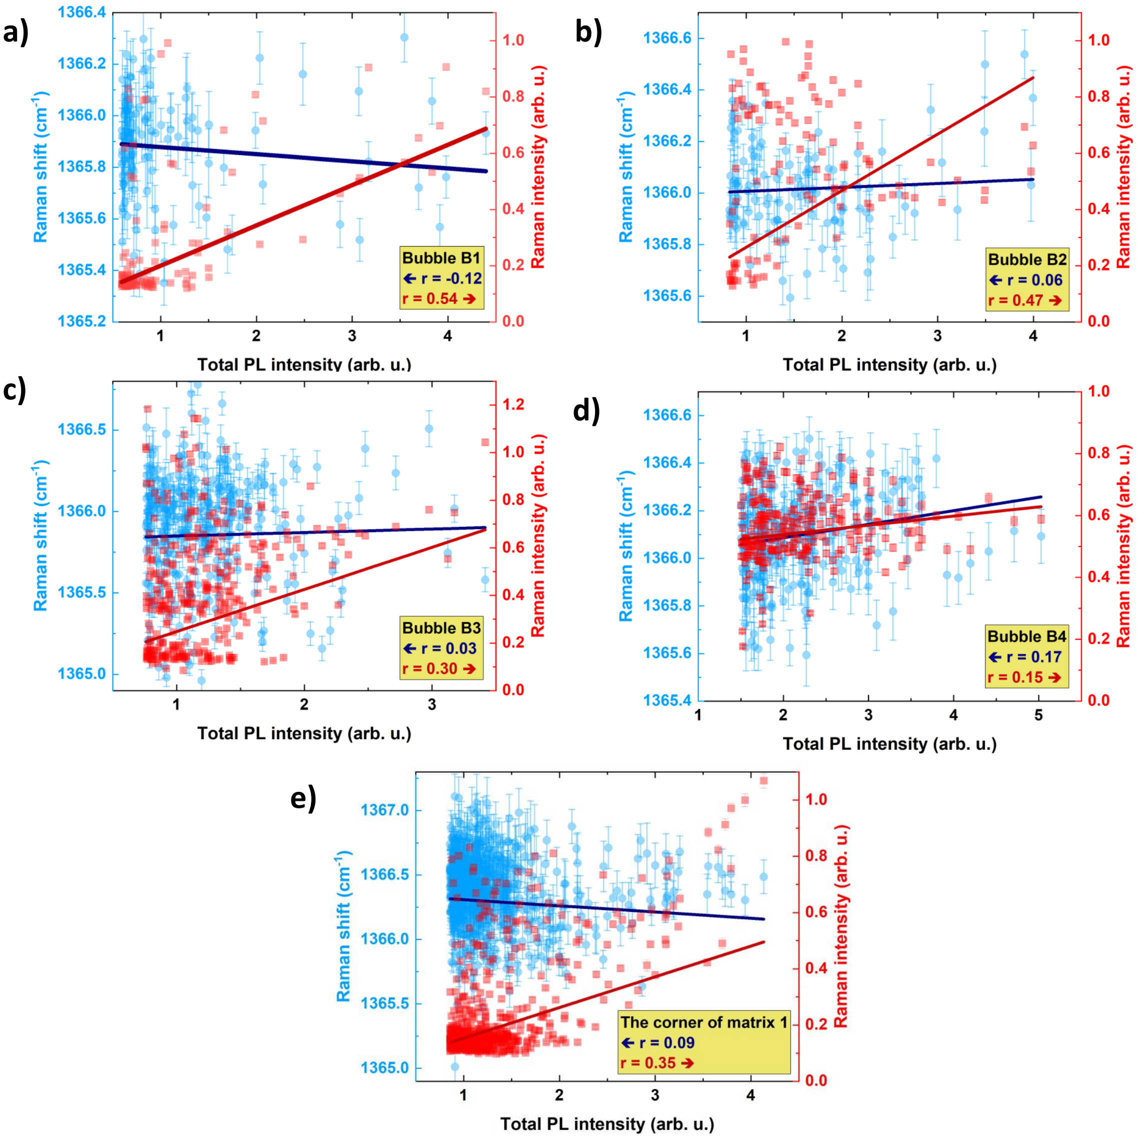


Figure S3: Dependencies of the total PL intensity on vibrational properties of hBN in mapped areas.

Figure S3 presents the relationships between the total collected PL signal intensity and vibrational properties of hBN for five different mapped areas. As mentioned in the main text, only the top 25 % points of the highest intensity were included in the analysis to avoid the influence of background emission and to exclude points where color centers were not present. PL intensity correlates more strongly with Raman signal intensity than with Raman peak position. This leads us to the conclusion that interference effects are responsible for the enhancement of SPEs, and strain does not play any role here.

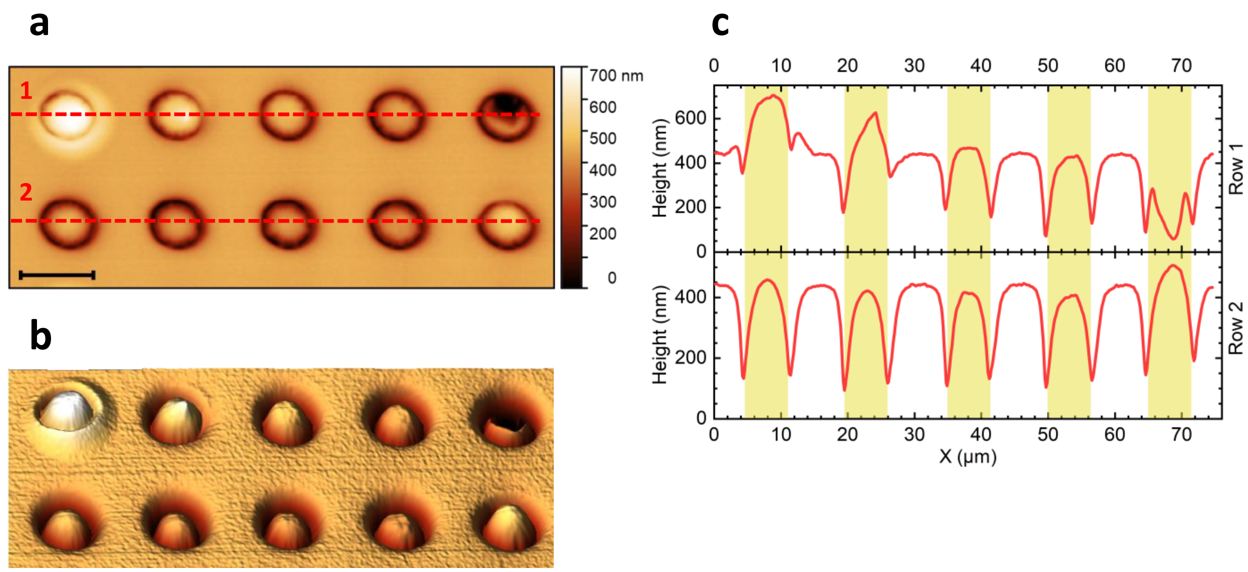


Figure S4: AFM characterization of a representative 2×5 matrix of regular bubbles obtained using a mask-based approach. a) and b) top and isometric views, respectively. The scale bar in a) is 10 µm. c) cross-sectional profiles along red dashed lines in a). Bubbles are marked by yellow.

Figure S4 presents AFM results on the 2×5 matrix of bubbles designed to be 6 µm in diameter-sized and separated by 15 µm. Similarly to the bubble matrix present in Figure 8, bubbles were created only in predefined holes; however, they still suffer from deviations. The bubble in the upper left corner expanded outside the designed areas and became higher than the others, while the one created in the upper right corner did not fully fill the resist-free area.

# Acknowledgement

This work was supported by the Polish National Science Centre under decisions 2020/39/D/ST7/02811 and 2022/45/N/ST7/03355.
